# Supplementary material for: SPIQ: Data-Free Per-Channel Static Input Quantization
Source: arXiv:2203.14642 source file (2022-03-28)
Supplement: Supplementary file 1 [file appendix.tex]

\clearpage
\appendix
